# Supplementary material for: Actions Speak What You Want: Provably Sample-Efficient Reinforcement Learning of the Quantal Stackelberg Equilibrium from Strategic Feedbacks
Source: arXiv:2307.14085 source file (2023-07-26)
Supplement: Supplementary file 1 [file bandit.tex]

\section{Proof of \Cref{lem:bandit} on MLE Estimator}\label{sec:proof-bandit}
Recall that $\hat\theta_\MLE$ minimizes the negative log likelihood 
\begin{align*}
    \cL^{(1)}_\cD(\theta) \defeq - \frac 1 T \sum_{t=1}^T \underbrace{\rbr{\eta \inp[]{\phi^t(b^t)} {\theta} - \log \rbr{\sum_{b'\in\cB}\exp\rbr{ \eta\inp[]{\phi^t(b')}{\theta} }}}}_{\ds \ell^t(\theta)},  
\end{align*}
where we abbreviate $\phi^{\alpha^t}(s^t, b)$ to $\phi^t(b)$ since both $\alpha^t$ and $s^t$ are uniquely determined by $t$. Showing the convergence of $\hat\theta_\MLE$ by directly working with $\cL^{(1)}_\cD(\theta)$ is not satisfactory since the Hessian of $\cL^{(1)}_\cD(\theta)$ is given by a direct computation
\begin{align*}
    \nabla^2\cL^{(1)}_\cD(\theta) = \frac 1 T \sum_{t=1}^T \eta^2 \EE_{b\sim\nu^{\pi^t, \theta}}\Bigsbr{
        \underbrace{\rbr{\phi^t(b) - \EE^{\nu^{\pi^t, \theta}}\phi^t}}_{\ds \psi^{t,\theta}(b)}
        \rbr{\phi^t(b) - \EE^{\nu^{\pi^t, \theta}}\phi^t}^\top }.
\end{align*}
Note that $\psi^{t, \theta}$ also depends on the choice of $\theta$, which makes the Hessian highly nonlinear. The strong convexity of this $\cL^{(1)}_\cD(\theta)$ is thus determined by the \textit{worst} $\theta$. Current techniques for lower bounding this Hessian hence suffers from a coefficient exponential in $\eta$. See Lemma Theorem 4 in \citet{shah2015estimation} where the upper bound depends on $\lambda_2(H)^{-1}$ and this eigenvalue can be $\exp(-\eta B_r)$. Or one can check from the proof of Lemma 3.1 in \citet{zhu2023principled} where the upper bound depends on $\gamma^{-1}$ with $\gamma=1/(2+\exp(-\eta B_r)+\exp(\eta B_r))$. This is not ideal for our setting since we may have a rather large $\eta$ if the follower has a higher level of rationality.
Therefore, our question is whether we can come up with an upper bound that only depends polynomial (later we will show that it is possible for linearity dependence) on $\eta$.

The key idea is replacing the negative log likelihood $\cL^{(1)}_\cD(\cdot)$ with some curve with constant Hessian $\EE_{\nu^{\pi^t, \theta^*}}[\psi^{t, \theta^*} {\psi^{t, \theta^*}}^\top]$ in the neighbourhood of $\theta^*$. Specifically, we first lower bound $\cL^{(1)}_\cD(\hat\theta_\MLE)-\cL^{(1)}_\cD(\theta^*)$ by the Hellinger distance $T^{-1}\cdot\sum_{t=1}^T D_\H^2(\nu^{\pi^t, \hat\theta_\MLE}, \nu^{\pi^t, \theta^*})$ and some $\cO(T^{-1})$ term. Then, a careful scrutiny of the Hellinger distance will show that $$D_\H^2(\nu^{\pi^t, \theta}, \nu^{\pi^t, \theta^*})\ge B_A^{-2} (\theta-\theta^*)^\top\EE^{\nu^{\pi^t, \theta^*}}[\psi^{t, \theta^*} {\psi^{t, \theta^*}}^\top](\theta-\theta^*).$$
To make the above discussion rigorous, we first invoke the following concentration Lemma.

Using \Cref{lem:freeman-variation} with $X_t = (-\ell^t(\theta) + \ell^t(\theta^*))/2$ and taking a union bound over $\theta\in\Theta$, we have with probability $1-\delta$ and for all $\theta\in\Theta$ that
\begin{align}
    \frac 1 2 \rbr{-\cL^{(1)}_\cD(\theta) + \cL^{(1)}_\cD(\theta^*)} &\le \frac 1 T \sum_{t=1}^T \log\EE^{\nu^{\pi^t, \theta^*}}\sbr{\sqrt\frac{\nu^{\pi^t,\theta}}{\nu^{\pi^t, \theta^*}}}  + \frac 1 T\log\rbr{\frac{\cN(\Theta, \epsilon)}{\delta}} + \epsilon\nend
    &\le - \frac 1 T \sum_{t=1}^T D_\H^2\rbr{\nu^{\pi^t, \theta}, \nu^{\pi^t, \theta^*}} + \frac 1 T\log\rbr{\frac{\cN(\Theta, \epsilon)}{\delta}} + \epsilon, \label{eq:KL-2-D_H}
\end{align}
where the first inequality holds since we take a $\epsilon$-covering net for each $\ell^t(\theta)$ over $\Theta$. Note that $\log(\cN(\Theta, \epsilon))$ only grows with $\log(\eta T)$ since $\ell^t(\theta)$ is $2\eta$-Lipschitz with respect to $\theta$. 
The second inequality holds by noting that $\log(x)\le x-1$ and by the definition of the Hellinger distance.
Note that the left hand side of \eqref{eq:KL-2-D_H} is lower bounded by $-\cL_\cD(\hat\theta)+\cL_\cD(\hat\theta_\MLE)$ if we plug in $\hat\theta\in \Theta$ by definition, which yields
\begin{align*}
    \frac 1 T \sum_{t=1}^T D_\H^2\rbr{\nu^{\pi^t, \hat\theta}, \nu^{\pi^t, \theta^*}} \le \frac 1 T\log\rbr{\frac{\cN(\Theta, \epsilon)}{\delta}} + \epsilon + \cL_\cD(\hat\theta)-\cL_\cD(\hat\theta_\MLE)
\end{align*}

We next lower bound the Hellinger distance with a quadratic form of $\hat\theta-\theta^*$.Invoking \Cref{lem:D_H-2-A^2}, we have that
\begin{align*}
    D_\H^2\rbr{\nu^{\pi^t, \hat\theta}, \nu^{\pi^t, \theta^*}} \ge \rbr{\frac{\eta}{1+\eta B_A}}^2\cdot \inp[\Big]{\nu^{\pi^t, \theta^*}}{ \rbr{A^{\pi^t, \hat\theta}-A^{\pi^t, \theta^*}}^2}, 
\end{align*}
where $B_A$ upper bound the advantage function $A$ and $A^{\pi^t, \theta}$ is a short hand of $A^{\pi^t, \theta}(s^t,)$. We further have
\begin{align*}
    \inp[\Big]{\nu^{\pi^t, \theta^*}}{ \rbr{A^{\pi^t, \hat\theta}-A^{\pi^t, \theta^*}}^2}
    &\ge \EE_{s^t}^{\pi^t, \theta^*}\rbr{\rbr{\EE_{s^t, b}^{\pi^t, \theta^*} - \EE_{s^t}^{\pi^t, \theta^*}}\sbr{A^{\pi^t, \hat\theta}-A^{\pi^t, \theta^*}}}^2\nend
    &= \EE_{s^t}^{\pi^t, \theta^*}\rbr{\rbr{\EE_{s^t, b}^{\pi^t, \theta^*} - \EE_{s^t}^{\pi^t, \theta^*}}\sbr{\inp[\big]{\phi^t(b)}{\hat\theta-\theta^*}}}^2, 
\end{align*}
where the inequality holds by the Jensen's inequality and the equality follows by 
invoking \Cref{lem:AQV-func diff} with $H=1$ and $\gamma=1$. Combining everything together, we have
\begin{align*}
    &(\hat\theta-\theta^*)^\top\Bigrbr{\underbrace{\frac 1 T\sum_{t=1}^T\EE^{\nu^{\pi^t, \theta^*}}[\psi^{t, \theta^*} {\psi^{t, \theta^*}}^\top]}_{\ds \Sigma_\cD^{\theta^*}}}
     (\hat\theta-\theta^*)\nend
    &\quad \le \bigrbr{\underbrace{\eta^{-1}+B_A}_{\ds C_\eta}}^2 \cdot 
     \rbr{\frac 1 T\log\rbr{\frac{\cN(\Theta, \epsilon)}{\delta}} + \epsilon+\cL_\cD(\hat\theta)-\cL_\cD(\hat\theta_\MLE)}, 
\end{align*}
Note that the Hellinger satisfies the exchangeability property and by swapping $\hat\theta$ with $\theta^*$, we also obtain
\begin{align*}
    &(\hat\theta-\theta^*)^\top\Bigrbr{\underbrace{\frac 1 T\sum_{t=1}^T\EE^{\nu^{\pi^t, \hat\theta}}[\psi^{t, \hat\theta} {\psi^{t, \hat\theta}}^\top]}_{\ds \Sigma_\cD^{\hat\theta}}}
    (\hat\theta-\theta^*)\nend
    &\quad \le \biggrbr{\underbrace{\frac{B_A}{1-\exp\rbr{-\eta B_A}}}_{\ds C_\eta}}^2 \cdot 
    \rbr{\frac 1 T\log\rbr{\frac{\cN(\Theta, \epsilon)}{\delta}} + \epsilon+\cL_\cD(\hat\theta)-\cL_\cD(\hat\theta_\MLE)}, 
\end{align*}
which proves the first statement \eqref{eq:bandit-ub-1}.
Note that for a finite follower's action set $\cB$ with $\abr{\cB}=K$, we actually have $\Sigma_\cD=\eta^{-2}\nabla^2\cL^{(1)}_\cD(\theta^*)= T^{-1}\sum_{t=1}^T \Phi^t \Xi^{t, \theta^*} (\Phi^t)^\top$ where $\Phi^t=[\phi^t(b_1),\dots, \phi^t(b_K)]$ and $\Xi^{t, \theta^*} = \diag(\nu^{\pi^t, \theta^*}) - (\nu^{\pi^t, \theta^*})(\nu^{\pi^t, \theta^*})^\top$.
For the Laplacian $L$ defined as
\begin{align*}
    L=T^{-1}\sum_{t=1}^T \Phi^t(KI-\ind\ind^\top)(\Phi^t)^\top, 
\end{align*}
we directly have for any $z\in\RR^d$ that
\begin{align*}
    z^\top \bar\Sigma_\cD z\ge \min\cbr{\frac{\lambda_d(\varPhi)}{\lambda_1(\bar\Sigma_\cD)}, \frac{K}{\min_{t\in[T]}\lambda_2(\Xi^{t, \theta^*})}} z^\top  L z, 
\end{align*}
where $\lambda_i(\cdot)$ is the $i$-th smallest eigen value and $\varPhi = T^{-1}\sum_{t=1}^T\Phi^t(\Phi^t)^\top$. 
Here, the first coefficient $\lambda_d(\varPhi)/\lambda_1(\bar\Sigma_\cD)$ is direct since $\lambda_d(L)\le \lambda_d(\varPhi)$, and the second coefficient follows by noting that $K\Xi^{t, \theta^*}/\lambda_2(\Xi^{t, \theta^*}) \succeq L$ where both $\Xi^{t, \theta^*}$ and $L$ shares the same null space $\rm{span}\{\ind\}$.
Hence, we complete the proof of \Cref{lem:bandit} by further plugging in $\epsilon=T^{-1}$.

\subsection{Follow up Discussion on \Cref{lem:bandit}}\label{sec:follow up on bandit}
We define $L_\cD$ as the standard Laplacian of the comparison feature graph, 
\begin{align*}
    L_\cD \defeq \frac 1 T \sum_{t=1}^T
    \rbr{\int_{\cB}\phi^t(b)\phi^t(b)^\top\rd b - \int_{\cB}\phi^t(b)\rd b \cdot \int_{\cB}\phi^t(b)^\top \rd b}.
\end{align*}
In particular, if $\cB$ is a finite action space with $K$ actions, we have $L_\cD = T^{-1}\sum_{t=1}^T \Phi^t(KI-\ind\ind^\top)(\Phi^t)^\top$ with $\Phi^t=[\phi^t(b_1),\dots, \phi^t(b_K)]$.
Moreover, for the standard Laplacian $L_\cD$, we have with probability at least $1-\delta$ that
    \begin{align}
        \bignbr{\hat\theta_\MLE-\theta^*}_{L_\cD}^2 \le \underbrace{\min\cbr{\frac{\lambda_d(\tilde\Phi) }{\lambda_1(\Sigma_\cD)}, \frac{K}{\min_{t\in[T]}\lambda_2(\Xi^{t, \theta^*})}}}_{\ds Z_\cD} C_\eta^2 \cdot 
        \frac 1 T\log\rbr{\frac{\cN(\Theta, 1/T)}{\delta}}, \label{eq:bandit-ub-2}
    \end{align}
    where $\Xi^{t, \theta^*} = \diag(\nu^{\pi^t, \theta^*}(\cdot\given s^t)) - (\nu^{\pi^t, \theta^*}(\cdot\given s^t))(\nu^{\pi^t, \theta^*}(\cdot\given s^t))^\top$ and $\tilde\Phi = T^{-1}\sum_{t=1}^T\Phi^t(\Phi^t)^\top$. If $\cB$ is a bounded continuous space, we still have guarantee for $Z_\cD= {\lambda_d(\tilde\Phi) }/{\lambda_1(\Sigma_\cD)}$ with $\tilde\Phi=\int_{\cB}\phi^t(b)\phi^t(b)^\top \rd b$.

To make a fair comparison with results in multiclass logistic regression, we consider $\pi^t$ and $s^t$ to be fixed across samples and the follower only has $K$ choices, which can be thought of as leader using the same strategy and querying the same state all the time. As it turns out, our upper bound \eqref{eq:bandit-ub-2} improves upon the previous results in terms of the choice number $K$ and the coefficient regarding the inverse temperature $\eta$. Note that $\Xi^{t, \theta^*}=\eta^{-2}\nabla^2 \cL^{(1)}_\cD(\theta^*) = \nabla^2(-\log \sigma(\inp[]{\phi^{t}}{\theta^*}))$ with $\sigma(x)=\exp(x_1)/\sum_{k=1}^K\exp(x_k)$. Our construction of $\Xi^{t, \theta^*}$ thus matches the definition of $H$ in \citet{shah2015estimation}, which enables a direct comparison as the following.
\textbf{Firstly}, in terms of $K$, our result only depends linearly in  $K/\lambda_2(\Xi^{t, \theta^*})$ while previous results have a quadratic dependence, e.g., Theorem 4 in \citet{shah2015estimation} or Theorem 4.1 in \citet{zhu2023principled}.
\textbf{Secondly}, in terms of $\eta$, the coefficient in \eqref{eq:bandit-ub-2} matches the $\eta^{-2}$ one given by the lower bound as $\eta$ approaches $0$ \citep[Theorem 1, Note that as $\eta\rightarrow 0$, $1-\exp(-\eta B_A)\rightarrow B_A\eta$  and $\lambda_2(\Xi^{t, \theta^*})\rightarrow K^{-1}$ since $\nu^{\pi^t, \theta^*}$ tends to a uniform distribution]{shah2015estimation}. 
On the other hand, for a large $\eta$, we have $C_\eta\rightarrow 1$ and the dependence on $\eta$ actually comes from $\lambda_2(\Xi^{t, \theta^*})^{-1}$ which may be of order $\exp(\eta B_A)$ in the worst case. However, we remark that $\lambda_2(\Xi^{t, \theta^*})$ only depends on the \textit{true parameter} $\theta^*$, which makes significantly improvements over the $\lambda_2(H)$ used in Theorem 4 of \citet{shah2015estimation} where they require $\nabla^2(-\log\sigma(\inp[]{\phi^t}{\theta}))\succ H$ for all $\theta\in\Theta$.
% for two arm comparison 
\textbf{Thirdly}, we notice that allowing the leader to change her strategy is a blessing rather than a detriment for purpose of learning the follower's reward, which may at first looks conterintuitive. To make the point clear, we consider a fixed $\pi^t=\pi^1$ against a changing $\pi^t$ across samples while we fix the state $s^t=s^1$ and let $\phi^{\alpha^1}(s^1, b)=I$.
If we fix the leader's policy $\pi=\pi^1$, the first term in $Z_\cD$ blows up since $\Sigma_\cD$ has a null space $\spn(\ind)$ by noting that $\Sigma_\cD=\Xi^{t,\theta^*}$. Thus, the second term of $Z_\cD$ dominates and we have $Z_\cD=K\exp(-\eta B_A)$ in the worst case. However, if we allow $\pi^t$ to change across samples, it is much more likely that $\Sigma_\cD$ no longer has this null space $\spn(\ind)$ and if $\Sigma_\cD$ further has full coverage over the $d$-dimensional space, the minimum taken in $Z_\cD$ will ensure that the coefficient does not scale with $\eta$ anymore (or at least no worst than just considering the second term in $Z_\cD$ in the fixed $\pi$ case.) \todo{put this discussion in the appendix and give a brief comparison.}

Lastly, we remark on why we should care about the dependence on the follower's action space size and the inverse temperature. \textbf{Firstly}, although it has been shown that it is difficult for humans to comprehense multiple choices at the same time \citep{saaty2003magic, miller1956magical, kiger1984depth}, it is on the contrary a much simpler task for human to make a selection in a simple continuous choice space \todo{to be added}. \textbf{Secondly}, if we consider an MDP with multi-step choices, the rate $\exp(\eta B_A) T^{-1}$ that appears in \citet{zhu2023principled,shah2015estimation} becomes intolerable for large $H$ and $\eta$ when $B_A\approx H B_r$. 
Thankfully, the analysis in \Cref{lem:bandit} suggests a much tighter upper bound given by \eqref{eq:bandit-ub-1}, which is obtained by studying the localized curvature of $\cL^{(1)}_\cD(\cdot)$ around the true parameter $\theta^*$ instead of looking at the global convexity of $\cL^{(1)}_\cD(\cdot)$.  Given that $\Sigma_\cD$ is the Hessian of the log-likelihood evaluated at $\theta^*$ up to a polynomial factor in $\eta$, \eqref{eq:bandit-ub-1} indicates an information-theoretically flavored upper bound.
