# Supplementary material for: Actions Speak What You Want: Provably Sample-Efficient Reinforcement Learning of the Quantal Stackelberg Equilibrium from Strategic Feedbacks
Source: arXiv:2307.14085 source file (2023-07-26)
Supplement: Supplementary file 3 [file response_diff_linear.tex]

% We first invoke the upper bound for this TV distance in \eqref{eq:response decomposition} of \Cref{lem:performance diff} where we take $H=1$ for myopic follower and swap the position of $\theta^*$ and $\tilde\theta$ (by the exchangeability of the TV distance), 
% \begin{align}
%     &D_\TV\rbr{\nu^{\pi,\theta^*}(\cdot\given s) , \nu^{\pi,\tilde\theta}(\cdot\given s)} \nend
%     &\quad \le \eta \cdot {\EE_{s}^{\pi, \tilde\theta}\sbr{\abr{\rbr{\EE^{\pi, \tilde\theta}_{s, b}-\EE^{\pi, \tilde\theta}_{s}}\bigsbr{ \inp{\phi^{\pi}(s, b)}{\theta^*-\tilde\theta} }}}} \nend
%     & \qquad\quad + \frac 1 2 \eta^2  \cdot 
%     {\EE_{s}^{\pi, \tilde\theta}\sbr{ \exp\bigrbr{\eta\bigabr{A^{\pi,\tilde\theta}-A^{\pi,\theta^*}}}\cdot \bigabr{A^{\pi,\tilde\theta} - A^{\pi, \theta^*}}^2}}\nend
%     &\quad \le \eta  \cdot \underbrace{\sqrt{\EE_{s}^{\pi, \tilde\theta}\sbr{\rbr{\rbr{\EE^{\pi, \tilde\theta}_{s, b}-\EE^{\pi, \tilde\theta}_{s}}\bigsbr{ \inp{\phi^{\pi}(s, b)}{\theta^*-\tilde\theta} }}^2 }}}_{\dr (i)} \nend
%     & \qquad\quad + \frac 1 2 \eta^2  \exp\rbr{2\eta B_A} \cdot 
%     {\EE_{s}^{\pi, \tilde\theta}\sbr{ \bigrbr{A^{\pi,\tilde\theta} - A^{\pi, \theta^*}}^2}},\label{eq:TV-ub-MLE} 
% \end{align}
% where the second inequality holds by using the Cauchy-Schwartz inequality and bounding the exponential term by its maximal value.
% By a standard variance and mean decomposition in the last quadratic term of \eqref{eq:TV-ub-MLE}, we obtain
% \begin{align}
%     \EE_{s}^{\pi, \tilde\theta}\sbr{ \bigrbr{A^{\pi,\tilde\theta} - A^{\pi, \theta^*}}^2}
%     & \le \EE_{s}^{\pi, \tilde\theta}\sbr{ \rbr{ \rbr{\EE^{\pi, \tilde\theta}_{s, b}-\EE^{\pi, \tilde\theta}_{s}}\sbr{A^{\pi,\tilde\theta} - A^{\pi, \theta^*}}}^2} + \rbr{\EE^{\pi, \tilde\theta}_{s}\sbr{A^{\pi,\tilde\theta} - A^{\pi, \theta^*}}}^2\nend
%     & =\underbrace{\EE_{s}^{\pi, \tilde\theta}\sbr{ \rbr{ \rbr{\EE^{\pi, \tilde\theta}_{s, b}-\EE^{\pi, \tilde\theta}_{s}}\sbr{\inp[\big]{\phi^{\pi}(s, b)}{\theta^*-\tilde\theta} }}^2}}_{\dr (i)^2} + \underbrace{\rbr{\EE^{\pi, \tilde\theta}_{s}\sbr{A^{\pi,\tilde\theta} - A^{\pi, \theta^*}}}^2}_{\dr (ii)}.
%     % &\le \EE_{s}^{\pi, \tilde\theta}\sbr{ \rbr{ \rbr{\EE^{\pi, \tilde\theta}_{s, b}-\EE^{\pi, \tilde\theta}_{s}}\sbr{\inp[\big]{\phi^{\pi}(s, b)}{\theta^*-\tilde\theta} }}^2}
%     % &\qquad + \underbrace{\rbr{ \rbr{\EE^{\pi, \theta^*}_{s}-\EE^{\pi, \tilde\theta}_{s}}\sbr{\inp[\big]{\phi^{\pi}(s, b)}{\theta^*-\tilde\theta} }}^2}_{\dr (iii)},
%     \label{eq:A-square-ub}
% \end{align}
% where the equality follows from \Cref{lem:AQV-func diff} on the difference in the advantage function
% % , and the last inequality holds by \Cref{lem:KL-ub} where we notice that $\kl\infdivx[\big]{\nu^{\pi, \tilde\theta}}{\nu^{\pi, \theta^*}} = \EE^{\pi, \tilde\theta}_{s}\bigsbr{A^{\pi,\tilde\theta} - A^{\pi, \theta^*}}$.
% Combining \eqref{eq:A-square-ub} with \eqref{eq:TV-ub-MLE}, we conclude that
% \begin{align}
%     D_\TV\rbr{\nu^{\pi,\theta^*}(\cdot\given s) , \nu^{\pi,\tilde\theta}(\cdot\given s)} &\le \eta \cdot {\dr(i)} + \frac{\eta^2\exp\rbr{2\eta B_A}}{2} \cdot \rbr{{\dr(i)}^2 + {\dr(ii)}}.\label{eq:TV-ub-offline}
% \end{align}
% It is straightforward to bound term (i) by guarantee of MLE.  By \eqref{eq:bandit-ub-2} in \Cref{lem:bandit}, we have
% \begin{align}
%     \bignbr{\theta^*-\tilde\theta_{\MLE}}_{{\Psi}}^2 \le \underbrace{\min\cbr{\frac{\lambda_d(\tilde\Phi) }{\lambda_1(\Sigma_{\cD})}, \frac{|\cB|}{\min_{t\in[T]}\lambda_2(\Xi^{t, \tilde\theta})}}}_{\ds Z_{\cD}} C_\eta^2 \cdot 
%         \frac 1 T\log\rbr{\frac{\cN(\Theta, 1/T)}{\delta}}, \label{eq:MLE-guarantee-offline}
% \end{align}
% where $C_\eta= {B_A}/\rbr{1-\exp\rbr{-\eta B_A}}$, $\Sigma_{\cD}=T^{-1}\cdot \sum_{t=1}^T\EE_{s^t}^{\nu^{\pi^t, \tilde\theta}}[\psi^{t, \tilde\theta} {\psi^{t, \tilde\theta}}^\top]$, $\psi^{t, \theta} =\phi^{t}(b) - \EE_{s^t}^{\nu^{\pi^t, \theta}}[\phi^t(b')]$, and 
% $\tilde\Phi^t=\int_{\cB}\phi^t(b)\phi^t(b)^\top \rd b$.
% Note if $\cB$ has infinitely many actions, the second term in $Z_{\cD}$ is meaningless and only the first term matters.
% If $\cB$ has finite actions, we define $\tilde\Phi^t=\sum_{b\in\cB}\phi^t(b)\phi^t(b)^\top$ and $\Xi^{t, \tilde\theta} = \diag(\nu^{\pi^t, \tilde\theta}(\cdot\given s^t)) - (\nu^{\pi^t, \tilde\theta}(\cdot\given s^t))(\nu^{\pi^t, \tilde\theta}(\cdot\given s^t))^\top$.

We have by \Cref{cor:response-diff-myopic} that 
\begin{align*}
    D_\TV\rbr{\nu(\cdot\given s), \tilde\nu(\cdot\given s)}
        &\le  \eta  \EE\sbr{\abr{(\tilde r^\pi(s, b) - r^\pi(s, b)) - \EE\bigsbr{\tilde r^\pi(s, b) - r^\pi(s, b)}}} \nend
        &\qquad + C^{(3)}\EE\sbr{\rbr{\rbr{\tilde r^\pi(s, b) -r^\pi(s, b)} - \EE\sbr{\tilde r^\pi(s, b) -r^\pi(s, b)}}^2}.
\end{align*}
% We define the weighted covariance matrix as
% \begin{align*}
%     \Sigma_{ s}^{\pi, \theta} \defeq \EE_{s}^{\pi, \theta} \sbr{\psi^{\pi,\theta}(s, b)\psi^{\pi,\theta}(s, b)^\top}\quad\text{where}\quad \psi^{\pi,\theta}(s, b) = \phi^{\pi}(s, b) - \EE_{s}^{\pi,\theta}\phi^{\pi}(s, \cdot).
% \end{align*}
% Under this definition, we introduce a nonnegative definite matrix $\Psi\in \SSS_+^{d}$ and write down the covariance term as
% \begin{align*}
%     &\EE\sbr{\rbr{\rbr{\tilde r^\pi(s, b) -r^\pi(s, b)} - \EE\sbr{\tilde r^\pi(s, b) -r^\pi(s, b)}}^2} \nend
%     &\quad = \bignbr{\theta^*-\tilde\theta}_{\Sigma_{ s}^{\pi, \tilde\theta}} = \nbr{\sqrt{\Psi}^{\dagger}\sqrt{\Psi}\rbr{\theta^*-\tilde\theta}}_{\Sigma_{ s}^{\pi, \tilde\theta}} \le \sqrt{\Bignbr{\Psi^{\dagger} \Sigma_{ s}^{\pi, \tilde\theta}}_\oper }\cdot \bignbr{\theta^*-\tilde\theta}_{\Psi} \le \sqrt{\trace\rbr{{\Psi}^{\dagger} \Sigma_{ s}^{\pi, \tilde\theta}}} \cdot \bignbr{\theta^*-\tilde\theta}_{\Psi}.
% \end{align*}
% where we recall from \Cref{lem:bandit} the definition of the weighted Laplacian of the comparison feature graph with respect to the offline data $\cD$ and parameter $\tilde\theta$ as $ \Sigma_\cD^{\theta}\defeq T^{-1} \sum_{t=1}^T
% \EE_{s^t}^{\pi^t, \theta}\bigsbr{\psi^{\pi^t, \theta}(s, b)\psi^{\pi^t, \theta}(s, b)^\top}$.
% Note that the operator norm is further bounded by the trace,
% \begin{align*}
%     \sqrt{\Bignbr{{\Psi}^{\dagger} \Sigma_{ s}^{\pi, \tilde\theta}}_\oper} 
%     &\le \sqrt{\trace\rbr{{\Psi}^{\dagger} \Sigma_{ s}^{\pi, \tilde\theta}}} \nend
%     &= \sqrt{\trace\rbr{\EE_{s}^{\pi, \tilde\theta}\sbr{ {\Psi}^\dagger \psi^{\pi,\tilde\theta}(s, b)\psi^{\pi,\tilde\theta}(s, b)^\top}}}\nend
%     & = \sqrt{\EE_{s}^{\pi, \tilde\theta}\sbr{\psi^{\pi,\tilde\theta}(s, b)^\top {\Psi}^\dagger  \psi^{\pi,\tilde\theta}(s, b)}}.
% \end{align*}
% We plug in the definition $\psi^{\pi,\tilde\theta}(s, b)=\phi^{\pi}(s, b) - \EE_{s}^{\pi,\tilde\theta}\phi^{\pi}(s, \cdot)$ and obtain
% \begin{align*}
%     &\sqrt{\EE_{s}^{\pi, \tilde\theta}\sbr{\psi^{\pi,\tilde\theta}(s, b)^\top {\Psi}^\dagger  \psi^{\pi,\tilde\theta}(s, b)}} = \underbrace{\sqrt{\EE_{s}^{{\pi,\tilde\theta}}\sbr{\phi^{\pi}(s,b)^\top {\Psi}^{\dagger}\phi^{\pi}(s,b)} -\bignbr{\EE_{s}^{{\pi,\tilde\theta}}\phi^{\pi}(s, b)}_{{\Psi}^{-1}}^2}}_{\ds \Upsilon_{s}^{\pi,\tilde\theta}}.
% \end{align*}
% Hence, we have for term (i) that  ${\dr (i)}\le 
% \Upsilon_{s}^{\pi,\tilde\theta}\cdot \bignbr{\theta^*-\tilde\theta}_{{\Psi}}$.
% % \begin{align}
% %     {\dr (i)} 
% %     &\le 
% %     \Upsilon_{s}^{\pi,\tilde\theta}\cdot \bignbr{\theta^*-\tilde\theta}_{{\Psi}}
% %     \le 2 \Upsilon_{s}^{\pi,\tilde\theta}\cdot \underbrace{\sqrt{Z_{\cD} C_\eta^2  \cdot \frac 1 T\log\rbr{\frac{\cN(\Theta, 1/T)}{\delta}} + \bignbr{\tilde\theta - \tilde\theta_{\MLE}}_{{\Psi}}^2}}_{\ds \zeta^{\tilde\theta}},\label{eq:myopic-(i)-ub}
% % \end{align}
% % on the success of \Cref{lem:bandit}. 
% % Here, the second inequality follows from the triangular inequaltiy, and the last inequality holds from \eqref{eq:MLE-guarantee-offline}.
% Now, we have addressed term (i) of \eqref{eq:TV-ub-offline} and it remains to show the upper bound for term (ii). Observe that under the quantal response model with logistic preference, term (ii) is nothing but just the squared KL divergence $\eta^{-2}\kl\infdivx[]{\nu^{\pi, \tilde\theta}(\cdot\given s)}{\nu^{\pi, \theta^*}(\cdot\given s)}^2$. Let $\Delta \theta=\tilde\theta - \theta^*$ and consider $\tilde\theta$ to be fixed. The Hessian of the KL divergence with respect to parameters in the second position is 
% \begin{align*}
%     \eta^{-2}\nabla_{\theta}^2 \kl\infdivx[]{\nu^{\pi, \tilde\theta}(\cdot\given s)}{\nu^{\pi, \theta}(\cdot\given s)} = \EE_s^{\pi,\theta} \sbr{\phi^\pi(s, b)\phi^\pi(s, b)^\top} - \EE_s^{\pi,\theta}\sbr{\phi^\pi(s, b)} \cdot \EE_s^{\pi,\theta}\sbr{\phi^\pi(s, b)}^\top = \Sigma_s^{\pi,\theta}.
% \end{align*}
% We observe that the KL divergence is strongly convex in the second parameter. Actually, for any test $x\in\RR^d$ and let $g(b)=\phi^\pi(s, \cdot)^\top x$, we have $x^\top \rbr{\eta^{-2}\nabla_{\theta}^2 \kl\infdivx[]{\nu^{\pi, \tilde\theta}(\cdot\given s)}{\nu^{\pi, \theta}(\cdot\given s)}} x = \Var^{\pi,\theta}[g(b)]$ and furthermore,
% \begin{align*}
%      \Var^{\pi,\theta}[g(b)]
%     \ge \exp(-2\eta B_A) \EE_s^{\pi, \tilde\theta}\sbr{\rbr{g(b) - \EE_s^{\pi,\theta}[g(b)]}^2} \ge \exp\rbr{-2\eta B_A} \Var^{\pi, \tilde\theta}[g(b)],
% \end{align*}
% which suggests that $\eta^{-2}\nabla_{\theta}^2 \kl\infdivx[]{\nu^{\pi, \tilde\theta}(\cdot\given s)}{\nu^{\pi, \theta}(\cdot\given s)}=\Sigma_s^{\pi,\theta}\succeq \exp(-2\eta B_A) \Sigma_s^{\pi,\tilde\theta}$. Actually, we can also swap $\theta$ and $\tilde\theta$ and obtain 
% \begin{align*}
%     \eta\exp(2\eta B_A) \Sigma_s^{\pi,\tilde\theta} \succeq \eta^{-}\nabla_{\theta}^2 \kl\infdivx[]{\nu^{\pi, \tilde\theta}(\cdot\given s)}{\nu^{\pi, \theta}(\cdot\given s)} \succeq \eta\exp(-2\eta B_A) \Sigma_s^{\pi,\tilde\theta} , \quad \forall \theta\in\Theta.
% \end{align*}
% Therefore, we can bound term (ii) simply by
% \begin{align*}
%     {\dr(ii)}\le \frac{\eta^2}{4} \exp\rbr{4\eta B_A} \bignbr{\theta^*-\tilde\theta}_{\Sigma_s^{\pi,\tilde\theta}}^4 \le  \frac{\eta^2}{4} \exp\rbr{4\eta B_A} \rbr{\Upsilon_{s}^{\pi,\tilde\theta}\cdot \bignbr{\theta^*-\tilde\theta}_{{\Psi}}}^4,
% \end{align*}
% where the last inequality holds by the same upper bound for term (i).
% Combining our results for both term (i) (ii), we have for \eqref{eq:TV-ub-offline} that
% \begin{align*}
%     &D_\TV\rbr{\nu^{\pi,\theta^*}(\cdot\given s) , \nu^{\pi,\tilde\theta}(\cdot\given s)} \nend
%     &\quad\le \eta \cdot {\dr(i)} + \frac{\eta^2\exp\rbr{2\eta B_A}}{2} \cdot \rbr{{\dr(i)}^2 + {\dr(ii)}}\nend
%     &\quad\le \eta \Upsilon_{s}^{\pi,\tilde\theta} \bignbr{\theta^*-\tilde\theta}_{{\Psi}} + \frac{\eta^2\exp\rbr{2\eta B_A}}{2} \rbr{\rbr{\Upsilon_{s}^{\pi,\tilde\theta} \bignbr{\theta^*-\tilde\theta}_{{\Psi}}}^2 + \frac{\eta^2}{4} \exp\rbr{4\eta B_A} \rbr{\Upsilon_{s}^{\pi,\tilde\theta} \bignbr{\theta^*-\tilde\theta}_{{\Psi}}}^4}.
% \end{align*}
% Now, we let $\Gamma^{(2)}(s;\pi_{s}, \tilde\theta) = \Upsilon_{s}^{\pi,\tilde\theta} \bignbr{\theta^*-\tilde\theta}_{{\Psi}} $ and 
% \begin{align*}
%     f(x) = \eta x + \frac{\eta^2\exp(2\eta B_A)}{2} x^2 + \frac{\eta^4\exp(6\eta B_A)}{8} x^4, 
% \end{align*}
% and just conclude that $D_\TV\bigrbr{\nu^{\pi_{s},\theta^*}(\cdot\given s) , \nu^{\pi_{s},\tilde\theta}(\cdot\given s)} \le f(\Gamma^{(2)}(s;\pi_{s}, \tilde\theta))$, 
% which completes the proof of \Cref{lem:response diff-myopic}. 
% % One can swap $\theta^*$ and $\$


% % \subsection{Follow up Discussion on \Cref{thm:PMLE-VI-myopic}}\label{sec:follow up on myopic offline}
% % \todo{comment on the use of the Laplacian, including why a standard $\sum\phi\phi^\top$ would fail. Also, comment on the use of $L_\cD$. }
